# Supplementary material for: ReaDiT Guidance: Control for Image and Video Generation using Diffusion Transformer Features
Source: arXiv:2609.04649 source file (2026-09-13)
Supplement: Supplementary file 1 [file X_supp.tex]

% \clearpage
% \appendix
% \resumetoc
% \setcounter{page}{1} % don't reset in arxiv version
% \renewcommand\thesection{\Alph{section}}
% \renewcommand\thesubsection{\thesection.\arabic{subsection}}
% \setcounter{section}{0}


% \begin{center}
%     {\Large \bfseries ReaDiT Guidance: Control for Image and Video Generation using Diffusion Transformer Features \par}
%     \vspace{1.0em}
%     {\Large \bfseries Supplementary Material \par}
%     % \vspace{1.0em}
% \end{center}

% \renewcommand{\contentsname}{\noindent\normalsize\textbf{Table of Contents}\vspace{-2.5em}}
% % \hypersetup{linkcolor=eccvblue}
% \begingroup
% \let\clearpage\relax
% \setlength{\parskip}{0pt}
% \hypersetup{linkcolor=eccvblue}
% \small                          % smaller font for TOC entries
% \setcounter{tocdepth}{3}
% \tableofcontents
% \endgroup
\clearpage
% \resumetoc % see https://stackoverflow.com/a/78998571
% \setcounter{page}{1} % don't reset in arxiv version
\renewcommand\thesection{\Alph{section}}
\renewcommand\thesubsection{\thesection.\arabic{subsection}}
\setcounter{section}{0}
\section*{Appendix}
\setcounter{tocdepth}{3}
% \tableofcontents

\input{sup_material/Architecture Anaylsis & Training}
\input{sup_material/PCA_analysis}
\input{sup_material/More Image Results}
\input{sup_material/More Video Results}
\input{sup_material/Guidance Details}
\input{sup_material/Eval Setup}
\input{sup_material/User Study Details}
\input{sup_material/Prompts in the paper}
\input{sup_material/Licenses}

% {
%     \small
%     \bibliographystyle{splncs04}
%     \bibliography{main,vsbib}
% }
